# Supplementary material for: The role of water and steric constraints in the kinetics of cavity-ligand unbinding
Source: arXiv:1507.02985 ancillary file (2015-07-10)
Supplement: Supplementary file 1 [file si.pdf]

# Supporting Information

Tiwary, Mondal, Morrone and Berne

July 9, 2015

## 1 Simulation set-up for MD, metadynamics and umbrella sampling calculations

The model ligand used in this work is a  $C_{60}$  fullerene and the pocket is an ellipsoidal hole carved from a hydrophobic slab, all interacting via Lennard-Jones potentials and enclosed by a periodic box of explicit water. This system was introduced previously in Ref.[1]. The pocket sites are fixed and interact with the model ligand with a Lennard-Jones potential having  $\sigma = 0.4152$  nm, kept same for all interactions. The pocket itself comprises 2 types of atomic species, interacting with the ligand atoms (color red in Fig. 1 in main text) as described below.

1. cavity atoms (color orange in Fig. 1 in main text), with Lennard-Jones  $\epsilon=0.008$  kJ/mol.
2. wall atoms (color green in Fig. 1 in main text), with Lennard-Jones  $\epsilon=0.0024$  kJ/mol.

The solute-solvent interactions are represented by the geometric mean of the respective water and solute parameters. All simulations are performed in explicit TIP4P water [2] with the GROMACS 4.5.4 MD package[3], patched with the PLUMED plugin[4]. During the equilibration stage, temperature and pressure are controlled with the stochastic velocity rescaling thermostat [5] and Berendsen barostat[6]. The production runs were NVT (constant number, volume, temperature) with a temperature of 300K.

The PLUMED plugin [4] was used to carry out metadynamics and umbrella sampling calculations. An integration time-step of  $2fs$  was used for all unbiased MD as well as metadynamics runs.

## 2 Simulation details for umbrella sampling

We employed umbrella sampling simulation technique for independent test of the free energy surfaces obtained through metadynamics. The umbrella sampling protocol followed for the case when the ligand is sterically constrained, is identical to that reported in Ref. [1] and we refer the reader to that reference.

Here we report the protocol followed to get the two-dimensional free energy surfaces in the scenario when the ligand is free to roll in any direction. Specifically, we discretize along  $z$  direction in a range of  $z = 0.8$  to  $2.0$  nm at intervals of  $0.1$  nm and along  $\rho = \sqrt{x^2 + y^2}$  direction in the range  $\rho = 0$  to  $1.2$  nm at intervals of  $0.1$  nm. Here a value of  $\rho = 0$  implies that the ligand is in centrosymmetric orientation with the cavity and any positive value of  $\rho$  implies a deviation of the centrosymmetric arrangement of the ligand relative to pocket. Thus in the 2-dimensional reaction space there are a total of  $13 \times 13=169$  windows. We generate the initial configurations corresponding to each umbrella window by performing a steered MD (SMD) simulations along  $\rho$  for a given  $z$  window starting with a centrosymmetrical ( $\rho = 0$ ) orientation and subsequently collecting corresponding configurations from the resulting SMD trajectories for all desired  $\rho$  and  $z$  combinations. For each of the 169 windows, we used a two-dimensional harmonic restraining potential. We adopt harmonic restraints  $U=0.5K_\rho(\rho - \rho_0)^2 + 0.5K_z(z - z_0)^2$  with  $K_\rho=4500$  kJ/mol/nm<sup>2</sup> and  $K_z=4500$  kJ/mol/nm<sup>2</sup>. The values of  $K_\rho$  and  $K_z$  were chosen such that the distributions of the corresponding reaction coordinates around the desired  $\rho_0$  and  $z_0$  are Gaussian in nature and there is significant overlap among adjacent windows.

In Fig. 1a we provide the 2-d free energy obtained through umbrella sampling for the case when the ligand is free to move in any direction. This is virtually indistinguishable from the free energy obtained through metadynamics (see Fig. 4a in main text). A similar comparison for the case when the ligand is sterically constrained has already been provided in the main text (Fig. 2a). In Fig. 1b we give the 1-d free energy as a function of  $z$  obtained from umbrella sampling and metadynamics. The barrier can be

seen to be lower than the case reported in main text where the fullerene is sterically constrained (Fig 2a in main text).

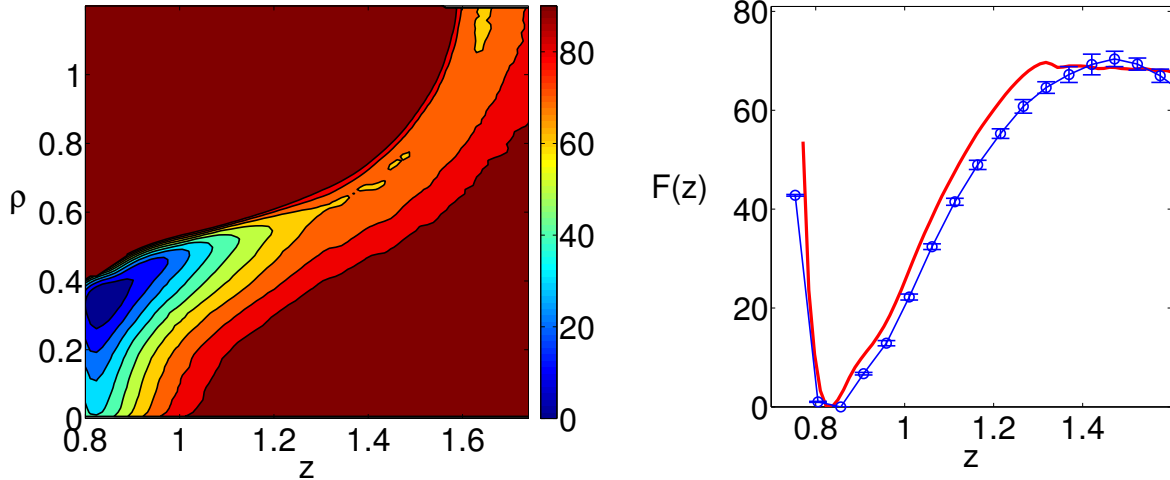

Figure 1: (a) Free energy profile from umbrella sampling for the case when the ligand is free to move in any direction, as a function of  $(z, \rho)$ . This is to be compared with Fig. 4(a) in the main text, which was obtained through metadynamics. (b) A comparison of the 1-d free energy as a function of  $z$  obtained from umbrella sampling (red line) and metadynamics (blue line with error bars). All energies are in kJ/mol and contours are separated by 10 kJ/mol.

### 3 Simulation details for metadynamics

In this section we provide details of CV, biasing kernel, biasing frequency and well-tempered metadynamics bias factor for various cases.

#### 3.1 Fullerene sterically constrained

##### 3.1.1 Metadynamics for free energy construction

For these calculations, bias was added on  $z$ -coordinate as the only CV using gaussian width of 0.02 nm. Gaussians were deposited every 0.6 ps, with a starting height of 2 kJ/mol and gradually decreased on the basis of well-tempered metadynamics biasing factor  $\gamma = 15$  [7]. Quartic restraining wall was used at  $z = 1.7$ .

##### 3.1.2 Metadynamics for rate constants

For these calculations, bias was added on  $z$ -coordinate as the only CV using gaussian width of 0.01 nm. Gaussians were deposited every 10 ps, with a starting height of 0.25 kJ/mol and gradually decreased on the basis of well-tempered metadynamics biasing factor  $\gamma = 10$  [7]. Since these calculations were stopped after first escape, no restraining walls were used.

#### 3.2 Fullerene free to move in any direction

##### 3.2.1 Metadynamics for free energy construction

For these calculations, bias was added on  $z$ - and the radial distance ( $\rho = \sqrt{x^2 + y^2}$ ) from the axis of symmetry as the two CVs, using gaussian widths of 0.03 nm and 0.01 nm respectively. Gaussians were deposited every 0.6 ps, with a starting height of 2 kJ/mol and gradually decreased on the basis of well-tempered metadynamics biasing factor  $\gamma = 15$  [7]. Quartic restraining walls were used at  $z = 2.1$  and  $\rho = 1.2$ .

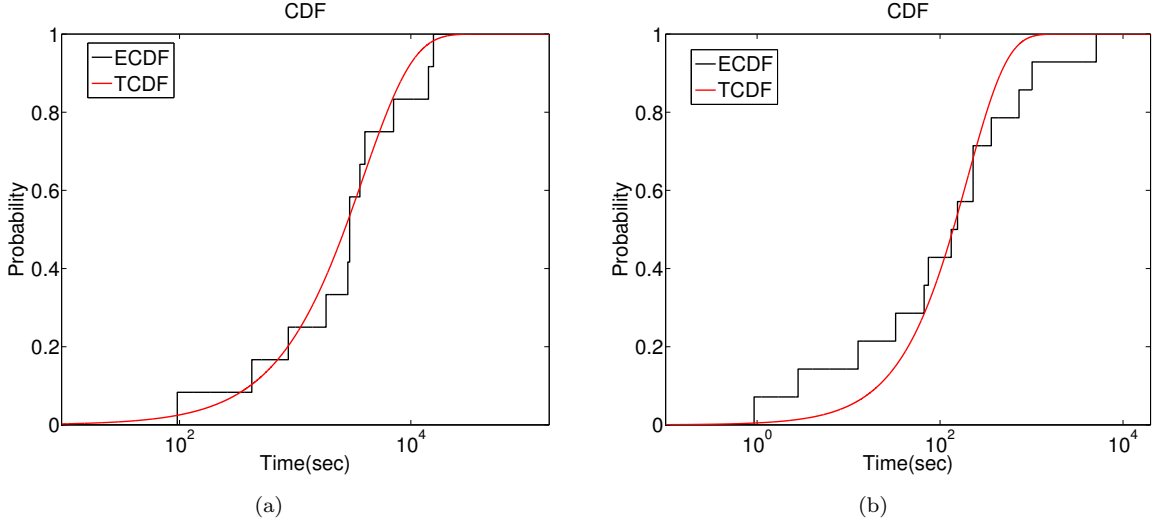

Figure 2: Poisson fit analysis for ligand (a) sterically constrained and (b) free to move in any direction. ECDF (black line) and TCDF (red line) denote empirical and theoretical (i.e. best fit) cumulative distribution functions respectively. The respective  $p$ -values for (a) and (b) are 0.72 and 0.64, which are well above the statistical threshold of 0.05.

### 3.2.2 Metadynamics for rate constants

For these calculations, bias was added on  $d = \sqrt{x^2 + y^2 + z^2}$ -coordinate as the only CV, using gaussian width of 0.03 nm. Gaussians were deposited every 10 ps, with a starting height of 1.2 kJ/mol and gradually decreased on the basis of well-tempered metadynamics biasing factor  $\gamma = 15$  [7]. Since these calculations were stopped after first escape, no restraining walls were used [7].

## 4 Kolmogorov-Smirnoff tests

The unbinding of a ligand from a binding pocket is a typical example of a rare event; the distribution of the associated transitions times is thus expected to be exponential, characteristic of a homogeneous Poisson process[9]. Comparing the empirical distribution of times obtained from metadynamics simulation using Eq. (1) in main text, with a theoretical exponential distribution provides an *a posteriori* assessment[10] of the fulfillment of requirements of the approach detailed in Ref. [11]. To compare the two distributions we proceed constructing the empirical cumulative distribution function (ECDF) of transition times obtained from simulations. Then the characteristic time of the corresponding theoretical Poisson process  $\tau$ , which is the timescale reported in the text, is obtained through a least squares fitting of the ECDF with the theoretical expression of a cumulative distribution function in the case of a homogeneous Poisson process (TCDF):

$$\text{TCDF} = 1 - \exp\left(-\frac{t}{\tau}\right) \quad (1)$$

This allow to obtain an estimate of the characteristic time of the Poisson process associated with the transition times obtained from simulation. To compare the theoretical (TCDF) and empirical (ECDF) distributions we carry out a Kolmogorov-Smirnoff (KS) test, in which we check the null hypothesis that the sample of transition times extracted from metadynamics and a large sample of times randomly generated according to an exponential probability distribution reflect the same underlying distribution.

As a quantitative measure of the similarity between the empirical and theoretical distributions we use the  $p$ -value associated to the KS statistic. The  $p$ -value represents the probability that the distribution of times extracted from metadynamics is obtained from the theoretical exponential distribution. In Ref. [10] this analysis is validated and discussed at length.

In Fig. 2, we provide the empirical and fitted cumulative distribution functions for both the cases considered in this work: (a) when the ligand is sterically constrained to roll along the axis of symmetry, (b) when the the ligand is free to move in any direction. The respective  $p$ -values respectively for the

two cases corresponding to the fitted timescales reported in the text, are 0.72 and 0.64, well above the threshold of 0.05[10, 12].

## Bibliography

- [1] Mondal J, Morrone JA, Berne BJ (2013) How hydrophobic drying forces impact the kinetics of molecular recognition. *Proceedings of the National Academy of Sciences* 110:13277.
- [2] Jorgensen WL, Chandrasekhar J, Madura JD, Impey RW, Klein ML (1983) Comparison of simple potential functions for simulating liquid water. *The Journal of chemical physics* 79(2):926–935.
- [3] Hess B, Kutzner C, Van Der Spoel D, Lindahl E (2008) Gromacs 4: algorithms for highly efficient, load-balanced, and scalable molecular simulation. *Journal of chemical theory and computation* 4(3):435–447.
- [4] Bonomi M et al. (2009) Plumed: A portable plugin for free-energy calculations with molecular dynamics. *Comp Phys Comm* 180(10):1961–1972.
- [5] Bussi G, Donadio D, Parrinello M (2007) Canonical sampling through velocity rescaling. *The Journal of chemical physics* 126(1):014101.
- [6] Berendsen HJ, Postma JPM, van Gunsteren WF, DiNola A, Haak J (1984) Molecular dynamics with coupling to an external bath. *The Journal of chemical physics* 81(8):3684–3690.
- [7] Barducci A, Bussi G, Parrinello M (2008) Well-tempered metadynamics: A smoothly converging and tunable free-energy method. *Phys Rev Lett* 100(2):020603–020606.
- [8] Tiwary P, Parrinello M (2015) A time-independent free energy estimator for metadynamics. *J Phys Chem B*.
- [9] Lelièvre T (2013) Two mathematical tools to analyze metastable stochastic processes (springer). pp. 791–810.
- [10] Salvalaglio M, Tiwary P, Parrinello M (2014) Assessing the reliability of the dynamics reconstructed from metadynamics. *J Chem Theory Comp* 10(4):1420–1425.
- [11] Tiwary P, Parrinello M (2013) From metadynamics to dynamics. *Physical review letters* 111(23):230602.
- [12] Tiwary P, Limongelli V, Salvalaglio M, Parrinello M (2015) Kinetics of protein–ligand unbinding: Predicting pathways, rates, and rate-limiting steps. *Proceedings of the National Academy of Sciences* 112(5):E386–E391.
